# Supplementary material for: Inverse Graphics GAN: Learning to Generate 3D Shapes from Unstructured 2D Data
Source: arXiv:2002.12674 source file (2020-02-28)
Supplement: Supplementary file 1 [file appendix.tex]

%%%%%%%%% ICML 2020 EXAMPLE LATEX SUBMISSION FILE %%%%%%%%%%%%%%%%%
%
%\documentclass[onecolumn]{article}
%
%% Recommended, but optional, packages for figures and better typesetting:
%\usepackage{microtype}
%\usepackage{graphicx}
%\usepackage{subcaption}
%\usepackage{float}
%\usepackage{amsmath}
%\usepackage{booktabs} % for professional tables
%\usepackage{makecell}
%% hyperref makes hyperlinks in the resulting PDF.
%% If your build breaks (sometimes temporarily if a hyperlink spans a page)
%% please comment out the following usepackage line and replace
%% \usepackage{icml2020} with \usepackage[nohyperref]{icml2020} above.
%\usepackage{hyperref}
%
%% Attempt to make hyperref and algorithmic work together better:
%\newcommand{\theHalgorithm}{\arabic{algorithm}}
%
%% Use the following line for the initial blind version submitted for review:
%\usepackage{icml2020}
%
%% If accepted, instead use the following line for the camera-ready submission:
%%\usepackage[accepted]{icml2020}
%
%% The \icmltitle you define below is probably too long as a header.
%% Therefore, a short form for the running title is supplied here:
%\icmltitlerunning{Inverse Graphics GAN: Supplemental Materials}
%
%\begin{document}
\onecolumn

%\twocolumn[
\icmltitle{Inverse Graphics GAN: Supplemental Material}

\appendix
\section{FID Scores Calculated with Inception Network Trained on ImageNet Classification}

In the main paper all FID scores were calculated using an Inception network which was trained to classify gray-scale ShapeNet renders that look similar to the training data used for all of our models.  Below we report, for the same set of experiments, FID scores calculated using the traditional ImageNet trained Inception network.

\begin{table}[H]
\caption{\label{tbl:maintable} Equivalent to Table 1 in the main paper.  ImageNet FID scores computed on ShapeNet objects (bathtubs, couches and chairs).   
\vspace{-1em}}
\begin{center}
 \begin{tabular}{c|ccc|ccc|cccc}
 \Xhline{3\arrayrulewidth}
 \# of Images&\multicolumn{3}{c|}{\bf $500$}&\multicolumn{3}{c|}{\bf One Per Model ($\approx 3000$)}&\multicolumn{3}{c}{\bf Unlimited}\\
 %\hline
 Dataset &{\bf Tubs}&{\bf Couches}&{\bf Chairs}&{\bf Tubs}&{\bf Couches}&{\bf Chairs}&{\bf Tubs}&{\bf Couches}&{\bf Chairs}&{\bf LVP}\\
 \Xhline{2\arrayrulewidth}
 2D-DCGAN&$356.9$&$324.6$&$291.9$&$211.0$&$156.5$&$196.8$&$210.1$&$117.8$&$78.8$&$101.5$\footnotemark[1]\\
\hline
 Visual Hull&$117.3$&$130.0$&$153.2$&$66.5$&$78.7$&$47.3$&$29.7$&$41.4$&${\bf22.0}$&$36.5$\\
\hline
 Absorbtion Only&$117.6$&$115.9$&${\bf110.7}$&$74.3$&$70.3$&$46.6$&$37.6$&$36.6$&$31.4$&$41.8$\\
 \Xhline{2\arrayrulewidth}
 IG-GAN (Ours)&${\bf 95.1}$&${\bf91.4}$&$131.4$&${\bf41.1}$&${\bf36.5}$&${\bf32.1}$&${\bf23.4}$&${\bf18.6}$&$22.6$&${\bf29.2}$\\
\Xhline{3\arrayrulewidth}
 \end{tabular}
\end{center}
\end{table}

\footnotetext[1]{A fair comparison to 2D-DCGAN is impossible, as the generator is trained on LVP (Limited View Point) data, but to facilitate easy comparison all FID evaluations are computed with same test data (which includes views from all 360$^{\circ}$).}

% \begin{table}[H]
%     \centering
%     \begin{tabular}{|c|c||c|c|c|c|}
%     \hline
%      Data & Size & DCGAN & AO & VH & Ours\\
%      \hline
%      \hline
%     Chairs & 500 & $291.9$ & ${\bf110.7}$ & $153.2$ & $131.4$ \\ 
%      \hline
%     Bathtubs & 500 & $356.9$ & $117.6$ & $117.3$ & ${\bf95.1}$\\ 
%      \hline
%     Couches & 500 & $324.6$ & $115.9$ & $130.0$ & ${\bf 91.4}$ \\ 
%      \hline
%     \hline 
%     Chairs & All & $196.8$ & $46.6$ & $47.3$ & ${\bf32.1}$ \\ 
%      \hline
%     Bathtubs & All & $211.0$ & $74.3$ & $66.5$ & ${\bf41.1}$ \\ 
%      \hline
%     Couches & All & $156.5$ & $70.3$ & $78.7$ & ${\bf36.5}$ \\ 
%      \hline
%     \hline 
%     Chairs & Unl. & $78.8$ & $31.4$ & ${\bf22.0}$ & $22.6$ \\ 
%      \hline
%     Bathtubs & Unl. & $210.1$ & $37.6$ & $29.7$ & ${\bf23.4}$ \\ 
%      \hline
%     Couches & Unl. & $117.8$ & $36.6$ & $41.4$ & ${\bf18.6}$ \\ 
%      \hline
%     \hline 
%      LVP & Unl. & $101.5$ & $41.8$ & $36.5$ & ${\bf29.2}$ \\ 
%  \hline
%     \end{tabular}
%     \caption{FID scores computed on ShapeNet objects (bathtubs, couches and chairs). FID scores use Inception weights pretrained on ImageNet}
% \end{table}

\begin{table}[H]
    \centering
        \caption{Equivalent to Table 2 in the main paper.  Ablation results without discriminator output matching (DOM) when training on \textcolor{red}{chairs}/\textcolor{blue}{couches} ``one per model'' datasets. We either fix the pre-trained neural renderer (``Fixed''), or continuing to train it during GAN training (``Retrained''). The generator samples fed to the discriminator are rendered using either OpenGL or the neural renderer. For reference, our model is equivalent to the Retrained OpenGL setup with the addition of the DOM loss and achieves FID scores \textcolor{red}{32.1}/\textcolor{blue}{36.5}.  FID scores calculated using an Inception network trained on ImageNet.}
    \begin{tabular}{c|c |c}
    & OpenGL & RenderNet \\ 
     \hline 
    Retrained & \textcolor{red}{$93.6$}/\textcolor{blue}{$146.6$} & \textcolor{red}{$58.1$}/\textcolor{blue}{$88.2$} \\ 
    Fixed & \textcolor{red}{$149.3$}/\textcolor{blue}{$238.6$} & \textcolor{red}{$61.6$}/\textcolor{blue}{$100.0$} \\ 
    \end{tabular}
\end{table}

\begin{table}[H]
    \centering
    \caption{Equivalent to Table 3 in the main paper.  Comparisons of neural renderer pre-trainings on different 3D shapes. FIDs are reported for the 'One per model' chairs. FID scores calculated using an Inception network trained on ImageNet.}
    \begin{tabular}{c|c c c c}
     & Chairs & Random & Tables \\ 
     \hline 
     \hline 
    Ours & $32.7$ & $31.4$ & $32.1$ \\ 
    Fixed & $43.0$ & $84.4$ & $69.5$ \\ 
    \end{tabular}
\end{table}

\section{A note on Emission-Absorption}
We chose to compare to the Absorption-only (AO) model from ~\citet{platosCave} and not the Emission-Absorption (EA) model.  The EA model was designed to incorporate color information into the differentiable rendering engine.  In addition to the occupancy/absorbtion value generated at each voxel, this model also generates one or more emission values at each voxel that can represent either 3-channel color, or a single grey-scale value.  The focus of our paper was only on shape, however, leaving color generation for future work.  Thus the underlying ShapeNet voxel data used in our experiments does not have any color channel information, and consists of only a single 0-1 occupancy value for each voxel.  Therefore, including the additional emission value would only result in providing the EA model additional freedom that it should not use when modeling the data.  In the following we show that if we assume that the model generates only a single occupancy channel and the emitted color is fixed globally, then the EA model naturally reduces to the AO model.

In ~\citet{platosCave} the expression
\begin{align*}
   \rho_{EA}(\textbf{v}) = \frac{\sum_{i=1}^{n_z} v_{a,i} v_{e,i} \prod_{j=1}^i (1-v_{a,j})} {\sum_{i=1}^{n_z} v_{a,i} \prod_{j=1}^i (1-v_{a,j}) + \epsilon} \left[ 1- \prod_{j=1}^{n_z} (1-v_{a,j}) \right]
\end{align*}
is used for the Emission-Absorption model, where $v_{e,j}$ denotes the emission coefficient, $v_{e,j}$ the absorption, $n_z$ the number of voxels along the chosen dimension and the index $j$ refers to the $j$-th occupancy of the 3D model along a straight line through the volume. The regularization parameter $\epsilon$ is chosen small to numerically stabilize the quotient. In the case of data generated from shape information alone, we can consider that all objects are perfectly white, which would equate to $v_{e,j} = 1$. In this case, the quotient 
\begin{align*}
    \frac{\sum_{i=1}^{n_z} v_{a,i} v_{e,i} \prod_{j=1}^i (1-v_{a,j})} {\sum_{i=1}^{n_z} v_{a,i} \prod_{j=1}^i (1-v_{a,j})}
\end{align*}
naturally reduces to one, leaving the expression
\begin{align*}
    \rho_{EA}(\textbf{v}) = 1- \prod_{j=1}^{n_z} (1-v_{a,j}),
\end{align*}
for the EA model, which is identical to the AO model. Hence, the two imaging models are the same in our setting of where images are obtained from 3D shapes with a single globally emitted color.

\section{Random Samples from Each Model Trained on Each of the Datasets}
The rest of the supplemental contains a set of tables where each table contains random samples from one of the models trained on one of the datasets.  For each set of random samples we show black and white renders as well as normal map renders.  In each figure the view angle is held fixed across all samples in a single row, but each image represents a completely independently sampled underlying 3D model.  Note that we cannot show normal map renderers for 2D-DCGAN generations since the 2D-DCGAN only generates images, not 3D models. At the end we also show samples from the dataset rendered in the same way for comparison.

\begin{figure*}
    \begin{subfigure}[t]{.45\textwidth}
    \centering
    \includegraphics[width=\textwidth]{Images_appendix/Chairs/All/DCGAN/00000.jpg}
    \caption{2D-DCGAN}
    \vspace{1cm}
    \end{subfigure}
    \hfill
    \begin{subfigure}[t]{.45\textwidth}
    \centering
    \includegraphics[width=\textwidth]{Images_appendix/Chairs/All/baseline_0/00000_th_02.jpg}
    \caption{Absorption Only}
        \vspace{1cm}
    \end{subfigure}
    \begin{subfigure}[t]{.45\textwidth}
    \centering
    \includegraphics[width=\textwidth]{Images_appendix/Chairs/All/baseline_2/00000_th_02.jpg}
    \caption{Visual Hull}
        \vspace{1cm}
    \end{subfigure}
    \hfill
    \begin{subfigure}[t]{.45\textwidth}
    \centering
    \includegraphics[width=\textwidth]{Images_appendix/Chairs/All/REINFORCE/00000_th_02.jpg}
    \caption{IG-GAN (Ours)}
        \vspace{1cm}
    \end{subfigure}
    \caption{Samples from models trained on the Chairs data in the 'one sample per object' setting (6667 training images).}
\end{figure*}

\begin{figure*}
    \begin{subfigure}[t]{.45\textwidth}
    \centering
    \includegraphics[width=\textwidth]{Images_appendix/Chairs/All/baseline_0/00000_th_02_NM.jpg}
    \caption{Absorption Only}
        \vspace{1cm}
    \end{subfigure}
    \begin{subfigure}[t]{.45\textwidth}
    \centering
    \includegraphics[width=\textwidth]{Images_appendix/Chairs/All/baseline_2/00000_th_02_NM.jpg}
    \caption{Visual Hull}
        \vspace{1cm}
    \end{subfigure}
    \hfill
    \begin{subfigure}[t]{.45\textwidth}
    \centering
    \includegraphics[width=\textwidth]{Images_appendix/Chairs/All/REINFORCE/00000_th_02_NM.jpg}
    \caption{IG-GAN (Ours)}
        \vspace{1cm}
    \end{subfigure}
    \caption{Samples from models trained on the Chairs data in the 'one sample per object' setting (6667 training images), r,endered as normal maps.}
\end{figure*}

\begin{figure*}
    \begin{subfigure}[t]{.45\textwidth}
    \centering
    \includegraphics[width=\textwidth]{Images_appendix/Couches/All/DCGAN/00000.jpg}
    \caption{2D-DCGAN}
    \vspace{1cm}
    \end{subfigure}
    \hfill
    \begin{subfigure}[t]{.45\textwidth}
    \centering
    \includegraphics[width=\textwidth]{Images_appendix/Couches/All/baseline_0/00000_th_02.jpg}
    \caption{Absorption Only}
        \vspace{1cm}
    \end{subfigure}
    \begin{subfigure}[t]{.45\textwidth}
    \centering
    \includegraphics[width=\textwidth]{Images_appendix/Couches/All/baseline_2/00000_th_02.jpg}
    \caption{Visual Hull}
        \vspace{1cm}
    \end{subfigure}
    \hfill
    \begin{subfigure}[t]{.45\textwidth}
    \centering
    \includegraphics[width=\textwidth]{Images_appendix/Couches/All/REINFORCE/00000_th_02.jpg}
    \caption{IG-GAN (Ours)}
        \vspace{1cm}
    \end{subfigure}
    \caption{Samples from models trained on the Couches data in the 'one sample per object' setting (3173 training images).}
\end{figure*}

\begin{figure*}
    \begin{subfigure}[t]{.45\textwidth}
    \centering
    \includegraphics[width=\textwidth]{Images_appendix/Couches/All/baseline_0/00000_th_02_NM.jpg}
    \caption{Absorption Only}
        \vspace{1cm}
    \end{subfigure}
    \begin{subfigure}[t]{.45\textwidth}
    \centering
    \includegraphics[width=\textwidth]{Images_appendix/Couches/All/baseline_2/00000_th_02_NM.jpg}
    \caption{Visual Hull}
        \vspace{1cm}
    \end{subfigure}
    \hfill
    \begin{subfigure}[t]{.45\textwidth}
    \centering
    \includegraphics[width=\textwidth]{Images_appendix/Couches/All/REINFORCE/00000_th_02_NM.jpg}
    \caption{IG-GAN (Ours)}
        \vspace{1cm}
    \end{subfigure}
    \caption{Samples from models trained on the Couches data in the 'one sample per object' setting (3173 training images), rendered as normal maps.}
\end{figure*}

\begin{figure*}
    \begin{subfigure}[t]{.45\textwidth}
    \centering
    \includegraphics[width=\textwidth]{Images_appendix/Bathtubs/All/DCGAN/00000.jpg}
    \caption{2D-DCGAN}
    \vspace{1cm}
    \end{subfigure}
    \hfill
    \begin{subfigure}[t]{.45\textwidth}
    \centering
    \includegraphics[width=\textwidth]{Images_appendix/Bathtubs/All/baseline_0/00000_th_02.jpg}
    \caption{Absorption Only}
        \vspace{1cm}
    \end{subfigure}
    \begin{subfigure}[t]{.45\textwidth}
    \centering
    \includegraphics[width=\textwidth]{Images_appendix/Bathtubs/All/baseline_2/00000_th_02.jpg}
    \caption{Visual Hull}
        \vspace{1cm}
    \end{subfigure}
    \hfill
    \begin{subfigure}[t]{.45\textwidth}
    \centering
    \includegraphics[width=\textwidth]{Images_appendix/Bathtubs/All/REINFORCE/00000_th_02.jpg}
    \caption{IG-GAN (Ours)}
        \vspace{1cm}
    \end{subfigure}
    \caption{Samples from models trained on the Bathtubs data in the 'four samples per object' setting (3424 training images). With this small dataset, we were unable to get the 2D-DCGAN model to stably train.  The resulting mode collapse causes the unusual grey background, as well as the high FID scores seen in Table \ref{tbl:maintable}.}
\end{figure*}

\begin{figure*}
    \begin{subfigure}[t]{.45\textwidth}
    \centering
    \includegraphics[width=\textwidth]{Images_appendix/Bathtubs/All/baseline_0/00000_th_02_NM.jpg}
    \caption{Absorption Only}
        \vspace{1cm}
    \end{subfigure}
    \begin{subfigure}[t]{.45\textwidth}
    \centering
    \includegraphics[width=\textwidth]{Images_appendix/Bathtubs/All/baseline_2/00000_th_02_NM.jpg}
    \caption{Visual Hull}
        \vspace{1cm}
    \end{subfigure}
    \hfill
    \begin{subfigure}[t]{.45\textwidth}
    \centering
    \includegraphics[width=\textwidth]{Images_appendix/Bathtubs/All/REINFORCE/00000_th_02_NM.jpg}
    \caption{IG-GAN (Ours)}
        \vspace{1cm}
    \end{subfigure}
    \caption{Samples from models trained on the Bathtubs data in the 'four samples per object' setting (3424 training images), rendered as normal maps.}
\end{figure*}

\begin{figure*}
    \begin{subfigure}[t]{.45\textwidth}
    \centering
    \includegraphics[width=\textwidth]{Images_appendix/Chairs/Unlimited/DCGAN/00000.jpg}
    \caption{2D-DCGAN}
    \vspace{1cm}
    \end{subfigure}
    \hfill
    \begin{subfigure}[t]{.45\textwidth}
    \centering
    \includegraphics[width=\textwidth]{Images_appendix/Chairs/Unlimited/baseline_0/00000_th_02.jpg}
    \caption{Absorption Only}
        \vspace{1cm}
    \end{subfigure}
    \begin{subfigure}[t]{.45\textwidth}
    \centering
    \includegraphics[width=\textwidth]{Images_appendix/Chairs/Unlimited/baseline_2/00000_th_02.jpg}
    \caption{Visual Hull}
        \vspace{1cm}
    \end{subfigure}
    \hfill
    \begin{subfigure}[t]{.45\textwidth}
    \centering
    \includegraphics[width=\textwidth]{Images_appendix/Chairs/Unlimited/REINFORCE/00000_th_02.jpg}
    \caption{IG-GAN (Ours)}
        \vspace{1cm}
    \end{subfigure}
    \caption{Samples from models trained on the Chairs data in the 'unlimited' setting.}
\end{figure*}

\begin{figure*}
    \begin{subfigure}[t]{.45\textwidth}
    \centering
    \includegraphics[width=\textwidth]{Images_appendix/Chairs/Unlimited/baseline_0/00000_th_02_NM.jpg}
    \caption{Absorption Only}
        \vspace{1cm}
    \end{subfigure}
    \begin{subfigure}[t]{.45\textwidth}
    \centering
    \includegraphics[width=\textwidth]{Images_appendix/Chairs/Unlimited/baseline_2/00000_th_02_NM.jpg}
    \caption{Visual Hull}
        \vspace{1cm}
    \end{subfigure}
    \hfill
    \begin{subfigure}[t]{.45\textwidth}
    \centering
    \includegraphics[width=\textwidth]{Images_appendix/Chairs/Unlimited/REINFORCE/00000_th_02_NM.jpg}
    \caption{IG-GAN (Ours)}
        \vspace{1cm}
    \end{subfigure}
    \caption{Samples from models trained on the Chairs data in the 'unlimited' setting, rendered as normal maps.}
\end{figure*}

\begin{figure*}
    \begin{subfigure}[t]{.45\textwidth}
    \centering
    \includegraphics[width=\textwidth]{Images_appendix/Chairs/LimitedVP/DCGAN/00000.jpg}
    \caption{2D-DCGAN}
    \vspace{1cm}
    \end{subfigure}
    \hfill
    \begin{subfigure}[t]{.45\textwidth}
    \centering
    \includegraphics[width=\textwidth]{Images_appendix/Chairs/LimitedVP/baseline_0/00000_th_02.jpg}
    \caption{Absorption Only}
        \vspace{1cm}
    \end{subfigure}
    \begin{subfigure}[t]{.45\textwidth}
    \centering
    \includegraphics[width=\textwidth]{Images_appendix/Chairs/LimitedVP/baseline_2/00000_th_02.jpg}
    \caption{Visual Hull}
        \vspace{1cm}
    \end{subfigure}
    \hfill
    \begin{subfigure}[t]{.45\textwidth}
    \centering
    \includegraphics[width=\textwidth]{Images_appendix/Chairs/LimitedVP/REINFORCE/00000_th_02.jpg}
    \caption{IG-GAN (Ours)}
        \vspace{1cm}
    \end{subfigure}
    \caption{Samples from models trained on the Chairs data in the 'unlimited' setting, using a limited viewpoint distribution.}
\end{figure*}

\begin{figure*}
    \begin{subfigure}[t]{.45\textwidth}
    \centering
    \includegraphics[width=\textwidth]{Images_appendix/Chairs/LimitedVP/baseline_0/00000_th_02_NM.jpg}
    \caption{Absorption Only}
        \vspace{1cm}
    \end{subfigure}
    \begin{subfigure}[t]{.45\textwidth}
    \centering
    \includegraphics[width=\textwidth]{Images_appendix/Chairs/LimitedVP/baseline_2/00000_th_02_NM.jpg}
    \caption{Visual Hull}
        \vspace{1cm}
    \end{subfigure}
    \hfill
    \begin{subfigure}[t]{.45\textwidth}
    \centering
    \includegraphics[width=\textwidth]{Images_appendix/Chairs/LimitedVP/REINFORCE/00000_th_02_NM.jpg}
    \caption{IG-GAN (Ours)}
        \vspace{1cm}
    \end{subfigure}
    \caption{Samples from models trained on the Chairs data in the 'unlimited' setting, using a limited viewpoint distribution, and rendered as normal maps.}
\end{figure*}

\begin{figure*}
    \begin{subfigure}[t]{.45\textwidth}
    \centering
    \includegraphics[width=\textwidth]{Images_appendix/Couches/Unlimited/DCGAN/00000.jpg}
    \caption{2D-DCGAN}
    \vspace{1cm}
    \end{subfigure}
    \hfill
    \begin{subfigure}[t]{.45\textwidth}
    \centering
    \includegraphics[width=\textwidth]{Images_appendix/Couches/Unlimited/baseline_0/00000_th_02.jpg}
    \caption{Absorption Only}
        \vspace{1cm}
    \end{subfigure}
    \begin{subfigure}[t]{.45\textwidth}
    \centering
    \includegraphics[width=\textwidth]{Images_appendix/Couches/Unlimited/baseline_2/00000_th_02.jpg}
    \caption{Visual Hull}
        \vspace{1cm}
    \end{subfigure}
    \hfill
    \begin{subfigure}[t]{.45\textwidth}
    \centering
    \includegraphics[width=\textwidth]{Images_appendix/Couches/Unlimited/REINFORCE/00000_th_02.jpg}
    \caption{IG-GAN (Ours)}
        \vspace{1cm}
    \end{subfigure}
    \caption{Samples from models trained on the Couches data in the 'unlimited' setting.}
\end{figure*}

\begin{figure*}
    \begin{subfigure}[t]{.45\textwidth}
    \centering
    \includegraphics[width=\textwidth]{Images_appendix/Couches/Unlimited/baseline_0/00000_th_02_NM.jpg}
    \caption{Absorption Only}
        \vspace{1cm}
    \end{subfigure}
    \begin{subfigure}[t]{.45\textwidth}
    \centering
    \includegraphics[width=\textwidth]{Images_appendix/Couches/Unlimited/baseline_2/00000_th_02_NM.jpg}
    \caption{Visual Hull}
        \vspace{1cm}
    \end{subfigure}
    \hfill
    \begin{subfigure}[t]{.45\textwidth}
    \centering
    \includegraphics[width=\textwidth]{Images_appendix/Couches/Unlimited/REINFORCE/00000_th_02_NM.jpg}
    \caption{IG-GAN (Ours)}
        \vspace{1cm}
    \end{subfigure}
    \caption{Samples from models trained on the Couches data in the 'unlimited' setting, rendered as normal maps.}
\end{figure*}

\begin{figure*}
    \begin{subfigure}[t]{.45\textwidth}
    \centering
    \includegraphics[width=\textwidth]{Images_appendix/Bathtubs/Unlimited/DCGAN/00000.jpg}
    \caption{2D-DCGAN}
    \vspace{1cm}
    \end{subfigure}
    \hfill
    \begin{subfigure}[t]{.45\textwidth}
    \centering
    \includegraphics[width=\textwidth]{Images_appendix/Bathtubs/Unlimited/baseline_0/00000_th_02.jpg}
    \caption{Absorption Only}
        \vspace{1cm}
    \end{subfigure}
    \begin{subfigure}[t]{.45\textwidth}
    \centering
    \includegraphics[width=\textwidth]{Images_appendix/Bathtubs/Unlimited/baseline_2/00000_th_02.jpg}
    \caption{Visual Hull}
        \vspace{1cm}
    \end{subfigure}
    \hfill
    \begin{subfigure}[t]{.45\textwidth}
    \centering
    \includegraphics[width=\textwidth]{Images_appendix/Bathtubs/Unlimited/REINFORCE/00000_th_02.jpg}
    \caption{IG-GAN (Ours)}
        \vspace{1cm}
    \end{subfigure}
    \caption{Samples from models trained on the Bathtubs data in the 'unlimited' setting.}
\end{figure*}

\begin{figure*}
    \begin{subfigure}[t]{.45\textwidth}
    \centering
    \includegraphics[width=\textwidth]{Images_appendix/Bathtubs/Unlimited/baseline_0/00000_th_02_NM.jpg}
    \caption{Absorption Only}
        \vspace{1cm}
    \end{subfigure}
    \begin{subfigure}[t]{.45\textwidth}
    \centering
    \includegraphics[width=\textwidth]{Images_appendix/Bathtubs/Unlimited/baseline_2/00000_th_02_NM.jpg}
    \caption{Visual Hull}
        \vspace{1cm}
    \end{subfigure}
    \hfill
    \begin{subfigure}[t]{.45\textwidth}
    \centering
    \includegraphics[width=\textwidth]{Images_appendix/Bathtubs/Unlimited/REINFORCE/00000_th_02_NM.jpg}
    \caption{IG-GAN (Ours)}
        \vspace{1cm}
    \end{subfigure}
    \caption{Samples from models trained on the Bathtubs data in the 'unlimited' setting,  rendered as normal maps.}
\end{figure*}

\begin{figure*}
    \begin{subfigure}[t]{.45\textwidth}
    \centering
    \includegraphics[width=\textwidth]{Images_appendix/dataset_vutils/Chairs/00000.jpg}
    \caption{Chairs}
        \vspace{1cm}
    \end{subfigure}
    \begin{subfigure}[t]{.45\textwidth}
    \centering
    \includegraphics[width=\textwidth]{Images_appendix/dataset_vutils/Couches/00000.jpg}
    \caption{Couches}
        \vspace{1cm}
    \end{subfigure}
    \hfill
    \begin{subfigure}[t]{.45\textwidth}
    \centering
    \includegraphics[width=\textwidth]{Images_appendix/dataset_vutils/Bathtubs/00000.jpg}
    \caption{Bathtubs}
        \vspace{1cm}
    \end{subfigure}
    \caption{Samples from the dataset, for reference.}
\end{figure*}

\begin{figure*}
    \begin{subfigure}[t]{.45\textwidth}
    \centering
    \includegraphics[width=\textwidth]{Images_appendix/dataset_vutils/Chairs/00000_NM.jpg}
    \caption{Chairs}
        \vspace{1cm}
    \end{subfigure}
    \begin{subfigure}[t]{.45\textwidth}
    \centering
    \includegraphics[width=\textwidth]{Images_appendix/dataset_vutils/Couches/00000_NM.jpg}
    \caption{Couches}
        \vspace{1cm}
    \end{subfigure}
    \hfill
    \begin{subfigure}[t]{.45\textwidth}
    \centering
    \includegraphics[width=\textwidth]{Images_appendix/dataset_vutils/Bathtubs/00000_NM.jpg}
    \caption{Bathtubs}
        \vspace{1cm}
    \end{subfigure}
    \caption{Samples from the actual data, rendered as normal map for reference.}
\end{figure*}

%\clearpage
%\bibliography{main}
%\bibliographystyle{icml2020}
%
%
%\end{document}
